# Supplementary material for: Universal Lossless Compression of Graphical Data
Source: arXiv:1909.09844 source file (2019-09-21)
Supplement: Supplementary file 1 [file Appendix_BC_Entropy_Properties.tex]

\section{Proof of Theorem~\ref{thm:Gen-BC-entorpy-properties}}
\label{sec:proof-theorem-gen-BC-properties}

In this section we discuss some properties of the marked BC entropy and prove Theorem~\ref{thm:Gen-BC-entorpy-properties}. First, in Section~\ref{sec:BC-invariance}, we prove that $\bchover$ and $\bchunder$ are  well defined, i.e. they are invariant under the specific choice of the sequences $\bm_n$ and $\bu_n$. 
Note that \eqref{eq:log-mG-n-bmn-m-log} together with the fact that for any $\epsilon>0$ and $\mu \in \mP(\mG_*)$, $\mG^{(n)}_{\bm_n, \bu_n}(\mu, \epsilon) \subseteq \mG^{(n)}_{\bm_n, \bu_n}$, immediately implies $H(\pi) + \sum_{x \in \Xi} s(d_x)$ is an upper bound for both $\bchover$ and $\bchunder$.
Finally, in Section~\ref{sec:cond-BC-infty}, we discuss conditions under which the entropy is $-\infty$.

\subsection{Invariance}
\label{sec:BC-invariance}

We prove the invariance in two steps. First, in Proposition~\ref{prop:bch-invariant-mn}, we fix the sequence $\bu_n$ and show invariance under the change of the sequence $\bm_n$. Later, in Proposition~\ref{prop:bch-invariant-mn}, we fix $\bm_n$ and show invariance under the change of the sequence $\bu_n$. 

\begin{prop}
\label{prop:bch-invariant-mn}
Assume $\mu \in \mP(\mGb_*)$ is given such that $0<\deg_x(\mu) <\infty$ for all $x \in \edgemark$ and $\vtype_t(\mu) > 0$ for all $t \in \vermark$. Additionally, assume that the degree vector $\bd=(d_x)_{x \in \edgemark}$ together with the probability distribution $\pi=(\pi_t)_{t \in \vermark}$ are given such that $0<d_x<\infty$ for all $x \in \edgemark$ and $\pi_t > 0$ for all $t \in \vermark$. 
Fix sequences $\bm_n, \tilde{\bm}_n$ and $\bu_n$ such that for all $x \in \edgemark$, $\lim_{n\rightarrow \infty} \bm_n(x)/n = \lim_{n \rightarrow \infty} \tilde{\bm}_n(x)/n = d_x/2$ and for all $t \in \vermark$, $\bu_n(t) / n \rightarrow \pi_t$. If $\bchover^{(1)}_{\bd,\pi}(\mu)$ is the entropy in definition~\ref{def:bch-color} resulting from the sequence $\bm_n$ and $\bchover^{(2)}_{\bd,\pi}(\mu)$ is the same object resulting from the sequence $\tilde{\bm}_n$ (where in both scenarios we use the sequence $\bu_n$ as the vertex mark counts),  we have $\bchover^{(1)}_{\bd,\pi}(\mu) = \bchover^{(2)}_{\bd,\pi}(\mu)$. Moreover, if $\bchunder^{(1)}_{\bd,\pi}(\mu)$ and $\bchunder^{(2)}_{\bd,\pi}(\mu)$ are defined similarly, we have $\bchunder^{(1)}_{\bd,\pi}(\mu) = \bchunder^{(2)}_{\bd,\pi}(\mu)$. 
\end{prop}

Before proving this proposition, we need the following lemma. The proof is postponed to after the proof of the above proposition.

\begin{lem}
  \label{lem:Gn-tilde-Gn-colored}
Assume that  $\mu \in \mP(\mGb_*)$ is given where $0<\deg_x(\mu) <\infty$ for all $x \in \Xi$. There exists a constant $\epsilon_0>0$ together with a  function $f: [0,\epsilon_0] \rightarrow \reals$ with $f(0) = 0$ and $f(\epsilon) > 0$ for $0< \epsilon\leq \epsilon_0$, which both depend only on $\mu$, such that the following is true: for an integer $n$, nonzero $\epsilon < \epsilon_0$, $\bm_n=(\bm_n(x))_{x \in \edgemark}$, $\tilde{\bm}_n=(\tilde{\bm}_n(x))_{x \in \edgemark}$, and $\bu_n = (\bu_n(t))_{t \in \vermark}$, if $|\bm_n(x) - \tilde{\bm}_n(x)| \leq f(\epsilon) n$ for all $x \in \edgemark$ and 
\begin{equation}
\label{eq:lemma-G-tildeG-n-condition}
  n \geq \frac{8 \left ( 2\frac{\sum_{x \in \Xi} \tilde{\bm}_n(x)}{n} + \epsilon |\Xi| \right )}{\epsilon^2},
\end{equation}
then, for all $\bG \in \mG^{(n)}_{\bm_n,\bu_n}(\mu, \epsilon)$ there exists a $\tilde{\bG} \in \mG^{(n)}_{\tilde{\bm}_n,\bu_n}$ such that 
\begin{equation*}
  \dlp(U(\bG), U(\tilde{\bG}) \leq 2 \epsilon.
\end{equation*}
Moreover, one can construct $\tilde{\bG}$ to have the following properties: for $x \in \Xi$, if $\bm_n(x) < \tilde{\bm}_n(x)$, then the set of edges in $\bG$ with mark $x$ is a subset of that of $\tilde{\bG}$. Furthermore, if $\bm_n(x) > \tilde{\bm}_n(x)$,  the set of edges of $\tilde{\bG}$ with mark $x$ is a subset of that of $\bG$. Finally, if $\bm_n(x) = \tilde{\bm}_n(x)$,  the set of edges of $\bG$ and $\tilde{\bG}$ with mark $x$ are identical. 
Further, there are at least 
\begin{equation*}
  \binom{\frac{\epsilon^2}{8} n^2}{\sum_{x: \bm_n(x) < \tilde{\bm}_n(x)} \tilde{\bm}_n(x) - \bm_n(x)}
\end{equation*}
many distinct marked graphs $\tilde{\bG}$ with the above properties. 
\end{lem}

\begin{proof}[Proof of Proposition~\ref{prop:bch-invariant-mn}]
  Take $\epsilon>0$ smaller than the $\epsilon_0$ introduced in  Lemma~\ref{lem:Gn-tilde-Gn-colored} above. 
Since $|\bm_n(x) - \tilde{\bm}_n(x)| / n \rightarrow 0$ for all $x \in \edgemark$, $|\bm_n(x) - \tilde{\bm}_n(x)| < f(\epsilon) n$ for $n$ large enough and the function $f$ in Lemma~\ref{lem:Gn-tilde-Gn-colored}. On the other hand, $\tilde{\bm}_n(x) / n \rightarrow d_x / 2$ for all $x \in \edgemark$, therefore the RHS of \eqref{eq:lemma-G-tildeG-n-condition} in Lemma~\ref{lem:Gn-tilde-Gn-colored} is bounded and we can choose $n$ large enough, such that \eqref{eq:lemma-G-tildeG-n-condition} is satisfied. As a result, 
for $n$ large enough the conditions of Lemma~\ref{lem:Gn-tilde-Gn-colored} are all  satisfied. Hence, if we take a graph $\bG_n \in \mG^{(n)}_{\bm_n,\bu_n}(\mu, \epsilon)$, we obtain at least 
\begin{equation*}
  \binom{\frac{\epsilon^2}{8} n^2}{\sum_{x: \bm_n(x) < \tilde{\bm}_n(x)} \tilde{\bm}_n(x) - \bm_n(x)}
\end{equation*}
many  $\tilde{\bG}_n \in \mG^{(n)}_{\tilde{\bm}_n,\bu_n}(\mu, 3 \epsilon)$. If we do this for all $\bG_n \in \mG^{(n)}_{\bm_n,\bu_n}(\mu, \epsilon)$, we get a subset of $\mG^{(n)}_{\tilde{\bm}_n,\bu_n}(\mu, 3\epsilon)$; however, a graph $\tilde{\bG}_n \in \mG^{(n)}_{\tilde{\bm}_n,\bu_n}(\mu, 3\epsilon)$ may be counted several times for different $G_n$'s.  Now, we give an upper bound on the number of $\bG_n$'s that could result in a single $\tilde{\bG}_n$.  Note that due to our construction in Lemma~\ref{lem:Gn-tilde-Gn-colored}, if $\bm_n(x) < \tilde{\bm}_n(x)$, the set of edges with color $x$ in $\bG_n$ is a subset of the set of edges with color $x$ in $\tilde{\bG}_n$. But there are
\begin{equation*}
  \binom{\tilde{\bm}_n(x)}{\tilde{\bm}_n(x) - \bm_n(x)}
\end{equation*}
many subsets of size $\bm_n(x)$ in the set of edges in $\tilde{\bG}_n$ with mark $x$. 
On the other hand, if $\bm_n(x) > \tilde{\bm}_n(x)$, the set of edges in $\bG_n$ with color $x$ is a superset of that of $\tilde{\bG}_n$. There are at most
\begin{equation*}
  \binom{\binom{n}{2}}{\bm_n(x) - \tilde{\bm}_n(x)}
\end{equation*}
many ways to choose these extra edges for $\bG_n$. Additionally, if $\bm_n(x) = \tilde{\bm}_n(x)$, the set of edges with color $x$ in $\bG_n$ and $\tilde{\bG}_n$ are identical. Hence, we have 
\begin{align*}
  \log |\mG^{(n)}_{\bm_n,\bu_n}(\mu, \epsilon)| &\leq \log |\mG^{(n)}_{ \tilde{\bm}_n,\bu_n}(\mu, 3\epsilon)| - \log \binom{\frac{\epsilon^2}{8} n^2}{\sum_{x \in \Xi} (\tilde{\bm}_n(x) - \bm_n(x) )^+} \\
  & \qquad + \sum_{x: \bm_n(x) < \tilde{\bm}_n(x)} \log \binom{\tilde{\bm}_n(x)}{\tilde{\bm}_n(x) - \bm_n(x)}  \\
  & \qquad + \sum_{x: \bm_n(x) \geq \tilde{\bm}_n(x)} \log \binom{\binom{n}{2}}{\bm_n(x) - \tilde{\bm}_n(x)} \\
\intertext{Using the inequality $(r/s)^s \leq \binom{r}{s} \leq (re/s)^s$ and Lemma~\ref{lem:upper-bound-on-G_n-m_mlogn-n} in Section~\ref{sec:generel-scheme}, with $\delta_n := \sum_{x:\tilde{\bm}_n(x) > \bm_n(x)} \tilde{\bm}_n(x) - \bm_n(x)$, } \\
&\leq \log |\mG^{(n)}_{\tilde{\bm}_n,\bu_n}(\mu, 3\epsilon) | - \delta_n \log \frac{\epsilon^2n^2}{8 \delta_n} \\
&\qquad + \sum_{x: \bm_n(x) < \tilde{\bm}_n(x)}(\tilde{\bm}_n(x) - \bm_n(x)) \log \frac{\tilde{\bm}_n(x)e}{\tilde{\bm}_n(x) - \bm_n(x)} \\
&\qquad + \sum_{x: \bm_n(x) > \tilde{\bm}_n(x)} ( \bm_n(x) - \tilde{\bm}_n(x)) \log n + n s \left ( \frac{2}{n} (\bm_n(x) - \tilde{\bm}_n(x)) \right ) \\
&= \log | \mG^{(n)}_{\tilde{\bm}_n,\bu_n}(\mu, 3\epsilon)| - \sum_{x \in \Xi} \tilde{\bm}_n(x) \log n + \sum_{x \in \Xi} \bm_n(x) \log n \\
& \qquad - n \left (\frac{\delta_n}{n} \log \frac{\epsilon^2}{8 \frac{\delta_n}{n} } \right ) \\
& \qquad + n \Bigg ( \sum_{x: \bm_n(x) < \tilde{\bm}_n(x)} \left ( \frac{\tilde{\bm}_n(x)}{n} - \frac{\bm_n(x)}{n} \right ) \log \frac{\tilde{\bm}_n(x) e}{n}  \\
& \qquad \qquad - \sum_{x: \bm_n(x) < \tilde{\bm}_n(x)} \left ( \frac{\tilde{\bm}_n(x)}{n} - \frac{\bm_n(x)}{n} \right ) \log \left ( \frac{\tilde{\bm}_n(x)}{n} - \frac{\bm_n(x)}{n} \right ) \Bigg ) \\
&\qquad + n \sum_{x: \bm_n(x) > \tilde{\bm}_n(x)}s \left ( \frac{2}{n} (\bm_n(x) - \tilde{\bm}_n(x)) \right )
\end{align*}
Since $|\frac{\bm_n(x)}{n} - \frac{\tilde{\bm}_n(x)}{n} | \rightarrow 0$, all terms on the RHS converge to zero after dividing by $n$  except for the first three terms. Therefore, if we move $\sum_{x \in \edgemark} \bm_n(x) \log n$ to the LHS, divide both sides by $n$ and take limsup, we have
\begin{equation*}
  \bchover_{\bd,\pi}^{(1)}(\mu, \epsilon) \leq \bchover^{(2)}_{\bd,\pi}(\mu, 3 \epsilon).
\end{equation*}
Following the same procedure and taking liminf instead of limsup we have
\begin{equation*}
    \bchunder_{\bd,\pi}^{(1)}(\mu, \epsilon) \leq \bchunder^{(2)}_{\bd,\pi}(\mu, 3 \epsilon).
\end{equation*}
Sending $\epsilon$ to zero we get 
\begin{equation*}
  \bchover_{\bd,\pi}^{(1)}(\mu) \leq \bchover^{(2)}_{\bd,\pi}(\mu) \qquad  \text{and} \qquad \bchunder_{\bd,\pi}^{(1)}(\mu) \leq \bchunder^{(2)}_{\bd,\pi}(\mu)
\end{equation*}
Repeating the above with $\bm_n$ and $\tilde{\bm}_n$ exchanged, we get the inequalities in the reverse direction which completes the proof.
\end{proof}

%{\color{red} the statement of the following lemma is very long which is not desirable, I am leaving it for now, but later I should make it shorter}

%{\color{red} substitute $\rho$ with $\mu$ in the following lemma}

\begin{proof}[Proof of Lemma~\ref{lem:Gn-tilde-Gn-colored}]
If $\epsilon_0 < 1/6$, since $\epsilon < \epsilon_0$, one can find an integer $k$ such that 
$\epsilon < 1/(1+k) < 1/k < 2 \epsilon$. For $r \in \nats$ and $x \in \Xi$, define $A^x_{k,r}$ to be the set of $[\bG', o'] \in \mGb_*$ such that $\deg_{\bG'}(o';x)  \geq 1$ and there are at most $r$ many vertices with distance at most $k$ from the root $o'$. Note that since elements of $\mGb_*$ are locally finite by definition, for all $k$ we have 
\begin{equation*}
  \{ [\bG', o'] \in \mGb_*: \deg_{\bG'}(o;x) \geq 1 \} = \bigcup_{r \geq 1} A^x_{k,r}.
\end{equation*}
As $\deg_x(\mu) > 0$ by assumption, we have 
\begin{equation*}
  \eta_x := \mu(\{[\bG', o']: \deg_{\bG'}(o';x) > 0 \}) > 0.
\end{equation*}
Thus, if we  choose $\epsilon_0 < \eta_x/2$,  continuity of the probability measure $\mu$ implies that there exists $r_x \in \nats$ such that $\mu(A^x_{k, r_x}) \geq 2 \epsilon$. On the other hand, as $\dlp(U(\bG), \mu) < \epsilon$, we have 
\begin{equation}
\label{eq:rho-Akr-U(G)}
  \mu (A^x_{k,r_x}) \leq U(\bG)((A^x_{k,r_x})^\epsilon) + \epsilon,
\end{equation}
where $(A^x_{k,r_x})^\epsilon$ is the $\epsilon$--extension of $A^x_{k, r_x}$. If $[\bG', o'] \in A^x_{k,r_x}$ and $\bar{d}_*([\bG', o'], [\bG'', o'']) \leq \epsilon$ for some $[\bG'', o''] \in \mGb_*$, $\epsilon < 1/(1+k)$ implies that $[\bG', o']_k \equiv [\bG'',o'']_k$. Therefore, $[\bG'',o'']$ has also at most $r_x$ vertices with distance at most $k$ from the root, and also $\deg_{\bG''}(o''; x) > 0$. This  means $([\bG'', o''] \in A^x_{k,r_x}$. Consequently, $(A^x_{k,r_x})^\epsilon = A^x_{k,r_x}$. This together with \eqref{eq:rho-Akr-U(G)} and $\mu(A^x_{k,r_x}) \geq 2\epsilon$ implies that 
\begin{equation*}
%  \label{eq:U(G)-Akr-bigger-than-epsilon}
  U(\bG)(A^x_{k,r_x}) \geq \epsilon.
\end{equation*}
As a result, if for $x \in \Xi$ we define
\begin{equation*}
  B_x := \{ i \in V(\bG): | \{ j\in V(\bG): d_{\bG}(i,j) \leq k \} | \leq r_x , \deg_{\bG}(i;x) \geq 1\},
\end{equation*}
we have 
\begin{equation}
  \label{eq:Bn-geq-epsilonn}
 |B_x| \geq \epsilon n.
\end{equation}
Furthermore, define 
\begin{equation*}
  \eta_0 := \mu ( \{ [\bG', o'] \in \mGb_*: \deg_{\bG'}(o') > 0 \}).
\end{equation*}
Note that $\eta_0 > 0$ by assumption.
Let $A_{k,r}$ be the set of $[\bG', o'] \in \mGb_*$ such that $\deg_{\bG'}(o') \geq 1$ and there are at most $r$ many vertices with distance at most $k$ from $o'$. A similar argument shows that if $\epsilon_0 < \eta_0 /2 $ (which is automatically satisfied when $\epsilon_0 < \eta_x$, since $\eta_x \leq \eta_0$), there exists an integer $r_0$ such that $U(\bG)(A_{k, r_0}) \geq \epsilon$. Thereby, with
\begin{equation*}
  B_0 := \{ i \in V(\bG): | \{ j\in V(\bG): d_{\bG}(i,j) \leq k \} | \leq r_0 , \deg_{\bG}(i) \geq 1\},
\end{equation*}
we have $ |B_0| \geq \epsilon n$.

Now, for each $x \in \edgemark$, we construct $\tilde{\bG}$ by adjusting the edges with mark $x$ so that their count becomes precisely $\tilde{\bm}_n(x)$. We do this without changing vertex marks. This is done for two categories of edge marks separately: those $x$ with $\bm_n(x) > \tilde{\bm}_n(x)$ and those with $\bm_n(x) < \tilde{\bm}_n(x)$ (when $\bm_n(x) = \tilde{\bm}_n(x)$, we leave the edges with mark $x$ unchanged).
For those $x$ such that $\bm_n(x) > \tilde{\bm}_n(x)$, we remove $\bm_n(x) - \tilde{\bm}_n(x)$ edges with at least one endpoint in $B_x$. For those $x$ such that $\bm_n(x) \leq \tilde{\bm}_n(x)$, we add $\tilde{\bm}_n(x) - \bm_n(x) $ edges with mark $x$ with both endpoints in $B_0$, in places where there is no edge in $\bG$. We first argue why this is possible. 
\begin{enumerate}
\item First consider $x$ such that $\bm_n(x) > \tilde{\bm}_n(x)$. Assume we impose the condition $f(\epsilon) < \frac{\epsilon}{2}$, which implies
\begin{equation}
\label{eq:f-epsilon-2-mnx-tmnx--epsilon2}
  \bm_n(x) - \tilde{\bm}_n(x) < \frac{\epsilon n}{2}.
\end{equation}
As we showed in \eqref{eq:Bn-geq-epsilonn}, $|B_x| \geq n \epsilon$ and each vertex in $B_x$ by definition has at least one edge with mark $x$ connected to it. Therefore, we go through vertices in $B_x$ one at a time and remove one edge with mark $x$ connected to each of them,  until the number of edges with mark $x$ in the graph reaches $\tilde{\bm}_n(x)$.  Inequality \eqref{eq:f-epsilon-2-mnx-tmnx--epsilon2} above and $|B_x| \geq n \epsilon$ together with the fact that each edge can use up at most two vertices in $B_x$ show that this procedure eventually succeeds.

\item Now, we turn to showing that we can add enough edges for  marks  $x$ when $\bm_n(x) < \tilde{\bm}_n(x)$. Note that there are at least 
\begin{equation*}
  \binom{|B_0|}{2} - \norm{\bm_n}_1 \geq \frac{|B_0|^2}{4} - \sum_{x \in \Xi} \left ( \tilde{\bm}_n(x) + f(\epsilon) n \right ) \geq \frac{\epsilon^2 n^2}{4} - \sum_{x \in \Xi} \left ( \tilde{\bm}_n(x) + f(\epsilon) n \right )
\end{equation*}
free slots in the graph with both endpoints in $B_0$.
On the other hand, we need to add totally
\begin{equation*}
  \sum_{x \in \Xi} \left (\tilde{\bm}_n(x)- \bm_n(x) \right)^+ \leq \sum_{x \in \Xi} \tilde{\bm}_n(x)
\end{equation*}
many edges to the graph to obtain $\tilde{\bG}$.
Hence, for us to be able to add these many edges, it suffices that 
\begin{equation*}
  \frac{\epsilon^2 n^2}{4} - \sum_{x \in \Xi} \left ( \tilde{\bm}_n(x) + f(\epsilon) n \right ) \geq \sum_{x \in \Xi} \tilde{\bm}_n(x).
\end{equation*}
If we require $f$ to satisfy $f(\epsilon) \leq \epsilon$, we get the above inequality by rearranging the terms in \eqref{eq:lemma-G-tildeG-n-condition}, which is assumed to hold.
% simplifying the above inequality yields to the following sufficient condition
% \begin{equation*}
%   n \geq \frac{8\left (2 \frac{\sum_{x \in \Xi} \tilde{\bm}_n(x)}{n} + \epsilon |\Xi|\right )}{\epsilon^2},
% \end{equation*}
% which is assumed to hold. 
This shows that our procedure is successful under the conditions stated. 
Moreover, with the above assumptions, we have 
\begin{equation*}
  \frac{\epsilon^2 n^2}{4} - \sum_{x \in \Xi} \left ( \tilde{\bm}_n(x) + f(\epsilon) n \right ) \geq \frac{\epsilon^2n^2}{4} - n \left ( 2 \frac{\sum_{x \in \edgemark} \tilde{\bm}_n(x)}{n} + \epsilon |\edgemark| \right ) \geq \frac{\epsilon^2 n^2}{8}.  
\end{equation*}
Thus, there are at least 
\begin{equation*}
  \binom{\frac{\epsilon^2n^2}{8}}{\sum_{x \in \Xi} (\tilde{\bm}_n(x) - \bm_n(x))^+}
\end{equation*}
overall possible choices for placing these $\sum_{x} (\tilde{\bm}_n(x) - \bm_n(x))^+$ edges, even without considering different possibilities for marking them. This means that there are these many possible distinct graphs as the outcome of our procedure. 
\end{enumerate}

So far we have given a recipe to construct $\tilde{\bG}$ from $\bG$ assuming that 
\begin{equation*}
  \epsilon_0 < \frac{1}{6} \wedge \min \left \{ \frac{\eta_x}{2}: x \in \Xi \right \},
\end{equation*}
and 
\begin{equation}
\label{eq:f-epsilon-condition-epsilon-2Xi}
  f(\epsilon) < \min \left \{ \frac{\epsilon}{2}, \epsilon \right \} = \frac{\epsilon}{2},
\end{equation}
and also $n \geq 8(2 \sum \tilde{\bm}_n(x) / n  + \epsilon |\Xi|)/\epsilon^2$.

Now, we show that $\dlp(U(\bG), U(\tilde{\bG})$ is no more than $2 \epsilon$. Let
\begin{equation*}
  C := \{ i \in V(\bG): (\bG, i)_{k-1} \equiv (\tilde{\bG}, i)_{k-1} \}.
\end{equation*}
Note that due to our definition, we remove mark $x$ edges with one endpoint in $B_x$, hence removing such an edge affects at most $r_x$ vertices up to depth $k-1$. On the other hand, adding an edge with both endpoints in $B_0$ can affect at most $2r_0$ vertices up to depth $k-1$. Therefore, if we define 
\begin{equation*}
  r_\text{max} := \max\{ r_x: x \in \Xi\} \vee r_0,
\end{equation*}
we have 
\begin{equation*}
  |C| \geq n - \left ( \sum_{x \in \Xi} |\bm_n(x) - \tilde{\bm}_n(x)| \right ) 2r_\text{max}.
\end{equation*}
Using Lemma~\ref{lem:local-isomorphism-LP-distance} in Section~\ref{sec:coding-step-1-restriction-max-degree},
\begin{equation*}
  \dlp(U(\bG), U(\bG')) \leq \max \left \{ \frac{1}{k} , \frac{1}{n} \left ( \sum_{x \in \Xi} |\bm_n(x) - \tilde{\bm}_n(x)| \right ) 2r_\text{max} \right \}.
\end{equation*}
Due our choice of $k$, $1/k < 2\epsilon$. Moreover, if we choose
\begin{equation*}
  f(\epsilon) \leq \frac{\epsilon}{|\edgemark| r_\text{max}},
\end{equation*}
the second term is also bounded by $2\epsilon$. This shows that $\dlp(U(\bG), U(\bG')) \leq 2\epsilon$. 
Comparing this to \eqref{eq:f-epsilon-condition-epsilon-2Xi}, we conclude that the choice 
\begin{equation*}
  f(\epsilon) := \frac{\epsilon}{|\edgemark| \max \{ 2, r_\text{max} \}},
\end{equation*}
satisfies all our requirements. 
Note that $r_x$ and $r_0$ only depend on $\mu$ and $\epsilon$, thereby the function $f$ only depends on $\mu$ and not $n$ or $\bG$. Also $\epsilon_0$ is a function of $\mu$ and $\edgemark$ only. Finally, since $f(\epsilon) \leq \epsilon /2$, $f(\epsilon) \rightarrow 0$ as $\epsilon \rightarrow 0$, and $f(\epsilon)>0$ for $\epsilon>0$.
\end{proof}

%\subsection{Vertex mark invariance}
%\label{sec:vert-mark-invar}

Now we turn to proving the invariance under the change of the sequence $\bu_n$. 

\begin{prop}
  \label{prop:bch-invariant-un}
Assume $\mu \in \mP(\mGb_*)$ is given such that $0<\deg_x(\mu) <\infty$ for all $x \in \Xi$ and $\vtype_t(\mu) > 0$ for all $t \in \vermark$.  Additionally, assume the degree vector $\bd=(d_x)_{x \in \edgemark}$ together with the probability distribution $\pi=(\pi_t)_{t \in \vermark}$ are given such that $0<d_x<\infty$ for all $x \in \edgemark$ and $\pi_t > 0$ for all $t \in \vermark$. 
Fix sequences $\bm_n, \bu_n,\tilde{\bu}_n$ such that $ \bm_n(x)/n \rightarrow d_x/2$ for all $x \in \edgemark$ and for all $t \in \vermark$, $\lim_{n \rightarrow \infty} \bu_n(t) / n = \lim_{n \rightarrow \infty} \tilde{\bu}_n(t) / n = \pi_t$. Let $\bchover^{(1)}_{\bd, \pi}(\mu)$ be the entropy in definition~\ref{def:bch-color} resulting from the sequence $\bu_n$ and $\bchover^{(2)}_{\bd, \pi}(\mu)$ is the same object resulting from the sequence $\tilde{\bu}_n$ (where in both scenarios we use $\bm_n$ for edge counts). Then, we have $\bchover^{(1)}_{\bd, \pi}(\mu) = \bchover^{(2)}_{\bd, \pi}(\mu)$. Moreover, if $\bchunder^{(1)}_{\bd, \pi}(\mu)$ and $\bchunder^{(2)}_{\bd, \pi}(\mu)$ are defined similarly, we also have $\bchunder^{(1)}_{\bd, \pi}(\mu) = \bchunder^{(2)}_{\bd, \pi}(\mu)$. 
\end{prop}

\marginpar{\color{red} Note that Definition ~\ref{def:bch-color}  discusses
$\bchover^{(1)}_{\bd, \pi}(\mu, \epsilon)$ and one needs to let $\epsilon \to 0$.}

\begin{rem}
  Although we have not assumed in the above statement that $d_x = \deg_x(\mu)$ for all $x \in \edgemark$, Proposition~\ref{prop:deg-not-match-bch-inf} in Appendix~\ref{sec:cond-BC-infty} implies that  if $d_x \neq \deg_x(\mu)$ for some $x \in \edgemark$, $\bchover^{(1)}_{\bd, \pi}(\mu) = \bchover^{(2)}_{\bd, \pi}(\mu) = \bchunder^{(1)}_{\bd, \pi}(\mu) = \bchunder^{(2)}_{\bd, \pi}(\mu) = -\infty$.
\end{rem}

\begin{proof}
Recall from \eqref{eq:vertype-probability} that $\vtype_t(\mu)$ is the probability under $\mu$ that the mark of the root is $t$. 
We claim that if $\pi_{\hat{t}} \neq \vtype_{\hat{t}}(\mu)$ for some $\hat{t} \in \vermark$, then $\bchover^{(1)}_{\bd, \pi}(\mu) = \bchover^{(2)}_{\bd, \pi}(\mu) = \bchunder^{(1)}_{\bd, \pi}(\mu) = \bchunder^{(2)}_{\bd, \pi}(\mu) = -\infty$. For instance, assume $\bchover^{(1)}_{\bd, \pi}(\mu) > -\infty$. A diagonalization argument implies that there exists an $M > -\infty$ together with sequences $n_k$ and $\epsilon_k$ such that as $k \rightarrow \infty$, $n_k \rightarrow \infty$ and $\epsilon_k \rightarrow 0$, and for all $k$.
\begin{equation*}
    \frac{\log |\mG^{(n_k)}_{\bm_{n_k}, \bu_{n_k}}(\mu, \epsilon_k)| - \norm{\bm_{n_k}}_1 \log n}{n_k} > M.
\end{equation*}
This in particular implies that the set $\mG^{(n_k)}_{\bm_{n_k}, \bu_{n_k}}(\mu, \epsilon_k)$ is not empty for every $k$. If $\bG_k$ is an arbitrary member of $\mG^{(n_k)}_{\bm_{n_k}, \bu_{n_k}}(\mu, \epsilon_k)$, since $\epsilon_k\rightarrow 0$, $\dlp(U(\bG_k), \mu) \rightarrow 0$. As the \LP metric metrizes the topology of weak convergence in $\mGb_*$, this means that $U(\bG_k)$ converges weakly to $\mu$. 
Now, define the function $f$ on $\mGb_*$ to be the indicator function of the mark of the root being $\hat{t}$, i.e. $f([\bG, o]) := \oneu{\tau_{\bG}(o) = \hat{t}}$. Since $f$ is bounded and continuous on $\mGb_*$ and $U(\bG_k) \Rightarrow \mu$, it must be the case that $\int f d U(\bG_k) \rightarrow \int f d \mu$. But $\int f dU(\bG_k) = \bu_{n_k}(\hat{t})/n_k$ while $\int f d \mu = \vtype_{\hat{t}}(\mu)$. This is a contradiction since $\bu_{n_k}(\hat{t})/n_k \rightarrow \pi_{\hat{t}} \neq \vtype_{\hat{t}}(\mu)$. Therefore, $\bchunder^{(1)}_{\bd, \pi}(\mu) \leq \bchover^{(1)}_{\bd, \pi}(\mu) = -\infty$. Similarly, $\bchunder^{(2)}_{\bd, \pi}(\mu) \leq \bchover^{(2)}_{\bd, \pi}(\mu) = -\infty$. Thus far, we have shown that if $\pi_{\hat{t}} \neq \vtype_{\hat{t}}(\mu)$ for some $\hat{t} \in \vermark$,  $\bchover^{(1)}_{\bd, \pi}(\mu) = \bchover^{(2)}_{\bd, \pi}(\mu) = \bchunder^{(1)}_{\bd, \pi}(\mu) = \bchunder^{(2)}_{\bd, \pi}(\mu) = -\infty$, and the statement of the above proposition holds.\footnote{It is fruitful to emphasize that a similar argument does not work for edge counts, i.e. to show that if $d_{x^*} \neq \deg_{x^*}(\mu)$ for some $x^* \in \edgemark$, $\bchover_{\bd, \pi}(\mu) = -\infty$. The reason is that although the function $f$ on $\mGb_*$ defined as $f([\bG, o]) = \deg_{\bG}(o;x^*)$ is continuous, it is not bounded. Thereby, one can not argue that the integral of $f$ against $U(\bG_k)$, which is $2 \bm_n(x^*) / n$, converges to $\int f d \mu = \deg_{x^*}(\mu)$. In fact, even if we truncate $f$ to make it bounded, by sending the truncation level to infinity and using monotone convergence theorem, we only get $\liminf \bm_n(x^*)/n \geq \deg_{x^*}(\mu)$. See Proposition~\ref{prop:deg-not-match-bch-inf} in Appendix~\ref{sec:cond-BC-infty}.} Hence, it remains to prove the statement under the assumption that $\pi_t = \vtype_t(\mu)$, for all $t \in \vermark$. 

Write $\vermark$ as $ \{t_1, \dots, t_{|\vermark|} \}$. Define
\begin{equation*}
  I^{(n)}_{t_1} := \{1, \dots, \bu_n(t_1) \},
\end{equation*}
and
\begin{equation*}
  I^{(n)}_{t_l} := \left \{ 1 + \sum_{i=1}^{l-1} \bu_n(t_i), \dots, \sum_{i=1}^l \bu_n(t_i)\right  \} \qquad 2 \leq l \leq |\vermark|.
\end{equation*}
Similarly, let
\begin{equation*}
  \tilde{I}^{(n)}_{t_1} := \{1, \dots, \tilde{\bu}_n(t_1) \},
\end{equation*}
and
\begin{equation*}
  \tilde{I}^{(n)}_{t_l} := \left \{ 1 + \sum_{i=1}^{l-1} \tilde{\bu}_n(t_i), \dots, \sum_{i=1}^l \tilde{\bu}_n(t_i)\right  \} \qquad 2 \leq l \leq |\vermark|.
\end{equation*}
Now, for an arbitrary graph $\bG \in \mG^{(n)}_{\bm_n, \bu_n}(\mu, \epsilon)$, 
one can find a permutation $\pi \in S_n$ such that in $\pi \bG$, all vertices in $I^{(n)}_{t_i}$ have mark $t_i$, for $1 \leq i \leq |\vermark|$. Then, $U(\pi \bG) = U(\bG)$. Let $\mG'^{(n)}_{\bm_n, \bu_n}$ be the subset of $\mG^{(n)}_{\bm_n, \bu_n}$ containing graphs in which all  vertices in $I^{(n)}_{t_i}$ have mark $t_i$,  $1 \leq i \leq |\vermark|$. Moreover, let $\mG'^{(n)}_{\bm_n, \bu_n}(\mu, \epsilon)$ be the set of graphs $\bG$ in $\mG'^{(n)}_{\bm_n, \bu_n}$ such that $\dlp(U(\bG), \mu) < \epsilon$. Let $\mG'^{(n)}_{\bm_n, \tilde{\bu}_n}$ and $\mG'^{(n)}_{\bm_n, \tilde{\bu}_n}(\mu, \epsilon)$ be defined similarly with $\bu_n$ being  replaced by  $\tilde{\bu}_n$. 

Let $S_{\bu_n}$ denote the subgroup of $S_n$ consisting of permutations $\pi$ such that $\pi I^{(n)}_{t_i} = I^{(n)}_{t_i}$, for $1 \leq i \leq |\vermark|$. Additionally, fix $M = \frac{n!}{\prod_{i=1}^{|\vermark|} \bu_n(t_i)!}$ permutations $\pi_1, \dots, \pi_M$ in $S_n$ such that $S_n$ is the disjoint union of $\pi_k S_{\bu_n}$ for $1 \leq k \leq M$. The above discussion then implies that $\mG^{(n)}_{\bm_n, \bu_n}(\mu, \epsilon)$ is the disjoint union of $\pi_k \mG'^{(n)}_{\bm_n, \bu_n}(\mu, \epsilon)$ for $1 \leq k \leq M$, where $\pi_k \mG'^{(n)}_{\bm_n, \bu_n}(\mu, \epsilon)$ denotes the action of $\pi_k$ on all graphs in $\mG'^{(n)}_{\bm_n, \bu_n}(\mu, \epsilon)$ (recall the notion of the action of a permutation on a graph from Section~\ref{sec:preliminaries}). This together with the fact that $\bu_n(t) / n \rightarrow \pi_t$ for all $t \in \vermark$ implies 
\begin{equation*}
  \log | \mG^{(n)}_{\bm_n, \bu_n}(\mu, \epsilon)| = \log |\mG'^{(n)}_{\bm_n, \bu_n}(\mu, \epsilon)| + nH(\pi) + o(n),
\end{equation*}
and similarly,
\begin{equation*}
  \log | \mG^{(n)}_{\bm_n, \tilde{\bu}_n}(\mu, \epsilon)| = \log |\mG'^{(n)}_{\bm_n, \tilde{\bu}_n}(\mu, \epsilon)| + nH(\pi) + o(n).
\end{equation*}
This shows that if we define 
\begin{equation*}
  \bchover'^{(1)}_{\bd, \pi}(\mu) := \lim_{\epsilon\downarrow 0} \limsup_{n\rightarrow \infty} \frac{\log |\mG'^{(n)}_{\bm_n, \bu_n}(\mu, \epsilon) | - \norm{\bm_n}_1\log n}{n},
\end{equation*}
and 
\begin{equation*}
  \bchover'^{(2)}_{\bd, \pi}(\mu) := \lim_{\epsilon\downarrow 0} \limsup_{n\rightarrow \infty} \frac{\log |\mG'^{(n)}_{\bm_n, \tilde{\bu}_n}(\mu, \epsilon) | - \norm{\bm_n}_1\log n}{n},
\end{equation*}
and  similarly $\bchunder'^{(1)}_{\bd, \pi}(\mu)$ and $\bchunder'^{(2)}_{\bd, \pi}(\mu)$, it suffices to show that $  \bchover'^{(1)}_{\bd, \pi}(\mu) =   \bchover'^{(2)}_{\bd, \pi}(\mu)$ and $\bchunder'^{(1)}_{\bd, \pi}(\mu) = \bchunder'^{(2)}_{\bd, \pi}(\mu)$. In order to do so, we define a mapping $F_n: \mG'^{(n)}_{\bm_n, \bu_n} \rightarrow \mG'^{(n)}_{\bm_n, \tilde{\bu}_n}$ in the following way:
given a graph $\bG \in \mG'^{(n)}_{\bm_n, \bu_n}$, for all vertices $1 \leq i \leq n$ in $\bG$, there is a unique $1 \leq j_i \leq |\vermark|$ such that $i \in \tilde{I}^{(n)}_{t_{j_i}}$. The mapping $F_n$ then changes the mark of all vertices $1 \leq i \leq n$ to $t_{j_i}$, and leaves edges and their marks untouched. 
See Figure~\ref{fig:Fn-vertex-mark-change} for an illustration.
Note that $F_n$ is a bijective mapping. 
 Our goal is to show that when $\epsilon$ is small enough and $n$ is large enough, for a sufficiently large fraction of graphs $\bG \in \mG'^{(n)}_{\bm_n, \bu_n}(\mu, \epsilon)$, $F_n(\bG)$ is contained in $\mG'^{(n)}_{\bm_n, \tilde{\bu}_n}(\mu, \epsilon')$, for $\epsilon'$ slightly larger than $\epsilon$. 

\begin{figure}
  \centering
  \begin{tikzpicture}
    \begin{scope}[xshift=-3cm,scale=0.7]
      \node[Node,label={above:1}] (n1) at (-1,1) {};
      \node[Node,label={above:2}] (n2) at (1,1) {};
      \node[Node2,label={below:3}] (n3) at (-1,-1) {};
      \node[Node2,label={below:4}] (n4) at (1,-1) {};
      \draw[Cyan,thick] (n2) -- (n1) -- (n4) -- (n3);
      \draw[Orange,densely dotted, very thick] (n2) -- (n3);
    \end{scope}
    \node at (0,0.5) {$F_n$};
    \draw[->] (-0.5,0) -- (0.5,0);
    \begin{scope}[xshift=3cm,scale=0.7]
      \node[Node,label={above:1}] (n1) at (-1,1) {};
      \node[Node2,label={above:2}] (n2) at (1,1) {};
      \node[Node2,label={below:3}] (n3) at (-1,-1) {};
      \node[Node2,label={below:4}] (n4) at (1,-1) {};
      \draw[Cyan,thick] (n2) -- (n1) -- (n4) -- (n3);
      \draw[Orange,densely dotted, very thick] (n2) -- (n3);
    \end{scope}
  \end{tikzpicture}
  \caption{\label{fig:Fn-vertex-mark-change} An illustration of the action of the function $F_n$. In this example, $n=4$,
$\edgemark = \{\text{\color{Cyan} Cyan (solid)}, \text{\color{Orange} Orange (dotted)} \}$,
$\vermark = \{t_1 = \bullet, t_2 = \blacksquare\}$, $\bu_n(t_1) = \bu_n(t_2) = 2$, $\tilde{\bu}_n(t_1) = 1, \tilde{\bu}_n(t_2) = 3$, $\bm_n({\color{Cyan} \text{Cyan}}) = 3$ and $\bm_n({\color{Orange} \text{Orange}}) = 1$. Note that the mark of vertex $2$ has changed from $\bullet$ to $\blacksquare$.}
\end{figure}

Let $\epsilon_0 = \frac{1}{6} \wedge \frac{1}{2} \min_{t \in \vermark} \pi_t$. Note that $\epsilon_0 > 0$ since by assumption $\pi_t > 0$ for all $t$. Choose $0 < \epsilon < \epsilon_0$ and fix an integer $k$ such that $\epsilon < 1/(1+k) < 1/k < 2 \epsilon$ (which is possible when $\epsilon< 1/6$). For $t \in \vermark$ and positive integer $r$, let $A^{t}_{k, r}$ be the set of $[\bG, o] \in \mGb_*$ such that the mark of the root is $t$ and there are at most $r$ many vertices up to depth $k$. Since the elements of $\mGb_*$ are locally finite, the probability of the mark of the root being $t$ is $\pi_t$, and $\epsilon<\min_{t \in \vermark} \pi_t$, we can choose $r_t$ such that $\mu(A^t_{k, r_t}) \geq \pi_t - \epsilon$. 
For a marked graph $\bG \in \mG'^{(n)}_{\bm_n, \bu_n}$ and $t \in \vermark$, let
\begin{equation*}
  J^{(n)}_t(\bG) := \{ i\in I^{(n)}_t: [\bG, i]_k \in A^t_{k, r_t} \}.
\end{equation*}

For $t \in \vermark$, let $Y^{(n)}_t = I^{(n)}_t \setminus \tilde{I}^{(n)}_t$, which is effectively the set of vertices with mark $t$ such that their mark is changed after applying $F_n$. Indeed, $Y^{(n)}_t$ only dependent on $\bu_n$ and $\tilde{\bu}_n$.
% (for instance, if $\vermark = \{a, b, c\}$, $n=5$, $\bu_n(a)= 1$, $\bu_n(b) = \bu_n(c) = 2$, $\tilde{\bu}_n(a)= \tilde{\bu}_n(b) = 2$ and $\tilde{\bu}_n(c) = 1$, then $Y^{(n)}_a = \emptyset$, $Y^{(n)}_b = \{2\}$ and $Y^{(n)}_c = \{4\}$). 
let $Y^{(n)} = \cup_{t \in \vermark} Y^{(n)}_t$. 
Moreover, due to the assumption that for all $t$, both $\bu_n(t)/ n$ and $\tilde{\bu}_n(t)/n$ converge to the same $\pi_t$, $|Y^{(n)}|=\sum_{t \in \vermark} |Y^{(n)}_t| = o(n)$. 
%which is essentially the set of vertices with mark $t$ in $\bG$ which do not have more than $r_t$ many nodes in their $k$--neighborhood. Note that if a vertex with mark $t$ which is going to change its mark (i.e. is in the set $Y^{(n)}_t$) is also in the set $J^{(n)}_t(\bG)$, since its local neighborhood up to depth $k$ does not contain more than a fixed number ($r_t$) many vertices, where $r_t$ does not depend on $n$, changing its color should not change $U(\bG)$ very much. To make this precise, 
We call $\bG \in \mG'^{(n)}_{\bm_n, \bu_n}$ to be \emph{good} if $Y^{(n)}_t \subseteq J^{(n)}_t(\bG)$ for all $ t\in \vermark$. Let $\bG' = F_n(\bG)$. Since the mark of a node $i \notin Y^{(n)}$ is unchanged after applying $F_n$, for a node $1 \leq j \leq n$, if $d_{\bG}(j, i) > k$ for all $i \in \cup_{t \in \vermark} Y^{(n)}_t$, the mark of all vertices in $(\bG,j)_k$ are unchanged after applying $F_n$ and $[\bG, j]_k \equiv [\bG', j]_k$. However, there are at least $n - \sum_{t \in \vermark} |Y^{(n)}_t| r_t$ many vertices satisfying this condition. Hence, using Lemma~\ref{lem:local-isomorphism-LP-distance} in Section~\ref{sec:coding-step-1-restriction-max-degree}, 
\begin{equation*}
  \dlp(U(\bG), U(\bG')) \leq \max \left \{ \frac{1}{k} , \frac{1}{n} \sum_{t \in \vermark} |Y^{(n)}_t|r_t \right \}.
\end{equation*}
Since $|Y^{(n)}_t| = o(n)$ for all $t \in \vermark$, we can choose $n$ large enough such that the above upper bound is no more than $1/k < 2 \epsilon$. To sum up, we have shown that if $\bG$ is a good graph,  $\dlp(U(\bG), U(F_n(\bG))) < 2 \epsilon$. This shows that if $\bG \in \mG'^{(n)}_{\bm_n, \bu_n}(\mu, \epsilon)$ is good, then $F_n(\bG) \in \mG'^{(n)}_{\bm_n, \tilde{\bu}_n}(\mu, 3\epsilon)$. 

Now we show that a sufficiently large fraction of  graphs in $\mG'^{(n)}_{\bm_n, \bu_n}(\mu, \epsilon)$ are good. For now, we assume that the set $\mG'^{(n)}_{\bm_n, \bu_n}(\mu, \epsilon)$ is not empty. Later we will discuss how to handle the case where $\mG'^{(n)}_{\bm_n, \bu_n}(\mu, \epsilon)$ is empty.
Let $\bG$ be drawn uniformly at random from the set $\mG'^{(n)}_{\bm_n, \bu_n}(\mu, \epsilon)$. Moreover, for $1 \leq i \leq n$, define the random variable $X_i$ to be 1 if $[\bG, i]_k \notin A^t_{k, r_t}$,  where $t$ is the mark of vertex $i$ in $\bG$. Otherwise, define $X_i$ to be zero. Invariance of $U(\bG)$ under vertex relabeling implies that for a permutation $\pi \in S_{\bu_n}$ and  $\bG \in \mG'^{(n)}_{\bm_n, \bu_n}(\mu, \epsilon)$, $\pi \bG \in \mG'^{(n)}_{\bm_n, \bu_n}(\mu, \epsilon)$. This means that 
\begin{equation}
  \label{eq:X-i-S-un-invariant}
  (X_{\pi(i)})_{1 \leq i \leq n} \stackrel{d}{=} (X_i)_{1 \leq i \leq n} \qquad \forall \pi \in S_{\bu_n},
\end{equation}
where $\stackrel{d}{=}$ denotes equality in distribution. Note that $\bG$ is good if and only for all  $i \in Y^{(n)}$, $X_i = 0$. On the other hand, if $\bG \in \mG'^{(n)}_{\bm_n, \bu_n}(\mu, \epsilon)$,  for all $t \in \vermark$, 
\begin{equation*}
  \mu(A^t_{k, r_t}) \leq U(\bG) \left ( \left(A^t_{k, r_t}\right)^\epsilon \right) + \epsilon.
\end{equation*}
But since $\epsilon < 1/(1+k)$, $(A^t_{k, r_t})^\epsilon = A^t_{k, r_t}$. By the definition of $r_t$, this means that $|J^{(n)}_t(\bG)| \geq n(\pi_t - 2 \epsilon$). 
Since $\epsilon< \pi_t / 2$, $\pi_t - 2 \epsilon > 0$ for all $t$.
As a result,
\begin{equation}
\label{eq:sum-Xi-upper-bound-li}
  \sum_{i \in I^{(n)}_t} X_i \leq \bu_n(t) - n \pi_t + 2n\epsilon \qquad \forall t \in \vermark.
\end{equation}
Now fix integers $l_1, \dots l_{|\vermark|}$ such that $0 \leq l_i \leq \bu_n(t_i) - n \pi_{t_i} + 2n\epsilon$ for all $1 \leq i \leq |\vermark|$. Then,  \eqref{eq:X-i-S-un-invariant} implies that  conditioned on the event $\sum_{j \in I^{(n)}_{t_i}} X_j = l_i$ for $1 \leq i \leq |\vermark|$, the sequence $X_1, \dots, X_n$ is uniformly distributed among the zero--one sequences with precisely $l_i$ many ones in $I^{(n)}_{t_i}$, for $1 \leq i \leq |\vermark|$.  
As $|Y^{(n)}| = o(n)$, we can choose $n$ large enough such that $l_i \leq \bu_n(t) - |Y^{(n)}_{t_i}|$, for all $1 \leq i \leq |\vermark|$. With such $n$, we have 
\begin{align*}
  \pr{X_j = 0\,\, \forall  j \in Y^{(n)} \Bigg| \sum_{j \in I^{(n)}_{t_i}} X_j = l_i, \forall 1 \leq i \leq |\vermark|} &= \frac{\prod_{i = 1}^{|\vermark|}\binom{\bu_n(t_i) - |Y^{(n)}_{t_i}|}{l_i}}{\prod_{i = 1}^{|\vermark|}\binom{\bu_n(t_i)}{l_i}} \\
&= \prod_{i = 1}^{|\vermark|} \frac{\bu_n(t_i) - |Y^{(n)}_{t_i}|}{\bu_n(t_i)} \times \dots \times \frac{\bu_n(t_i) - |Y^{(n)}_{t_i}| - l_i + 1}{\bu_n(t_i) - l_i + 1} \\
&\geq \prod_{i = 1}^{|\vermark|} \left ( \frac{\bu_n(t_i) - |Y^{(n)}_{t_i}| - l_i + 1}{\bu_n(t_i) - l_i + 1} \right )^{l_i} \\
&\geq \prod_{i = 1}^{|\vermark|} \left ( \frac{n(\pi_{t_i} - 2\epsilon) - |Y^{(n)}_{t_i}| + 1}{n(\pi_{t_i} - 2\epsilon) + 1} \right)^{\bu_n(t_i) - n(\pi_{t_i} - 2\epsilon)}
\end{align*}
where the last inequality follows from the fact that each term is decreasing in $l_i$ and $l_i \leq \bu_n(t_i) - n\pi_{t_i} +2n\epsilon$. Since this lower bound is uniform over $l_i$, we have 
\begin{equation}
  \label{eq:pr-G-good}
  \pr{\bG \text{ is good}} = \pr{X_j = 0 \,\, \forall j \in Y^{(n)}} \geq \prod_{i = 1}^{|\vermark|} \left ( \frac{n(\pi_{t_i} - 2\epsilon) - |Y^{(n)}_{t_i}| + 1}{n(\pi_{t_i} - 2\epsilon) + 1} \right)^{\bu_n(t_i) - n(\pi_{t_i} - 2\epsilon)} =: \alpha_n.
\end{equation}
As $\bG$ was chosen uniformly at random in $\mG'^{(n)}_{\bm_n, \bu_n}(\mu, \epsilon)$, this means that a $\alpha_n$ fraction of graphs in $\mG'^{(n)}_{\bm_n, \bu_n}(\mu, \epsilon)$ are good. This together with the fact that if $\bG$ is good, $F(\bG) \in \mG'^{(n)}_{\bm_n, \tilde{\bu}_n}(\mu, 3\epsilon)$ implies that 
\begin{align*}
  \log |\tilde{\bG}^{(n)}_{\bm_n, \tilde{\bu}_n} (\mu, 3\epsilon) | &\geq \log |\tilde{\bG}^{(n)}_{\bm_n, \bu_n} (\mu, \epsilon) | + \log \alpha_n  \\
&= \log |\tilde{\bG}^{(n)}_{\bm_n, \bu_n} (\mu, \epsilon) | + n \left ( \sum_{i=1}^{|\vermark|} \left ( \frac{\bu_n(t_i) - \pi_{t_i}}{n} +2\epsilon \right ) \log \left ( 1 - \frac{|Y^{(n)}_{t_i}|}{n(\pi_{t_i} - 2\epsilon) + 1} \right ) \right )
\end{align*}
Earlier we had made the assumption that $\mG'^{(n)}_{\bm_n, \bu_n}(\mu, \epsilon)$ is not empty to obtain the above inequality. But if $\mG'^{(n)}_{\bm_n, \bu_n}(\mu, \epsilon)$ is empty, the RHS is $-\infty$ and the above inequality still remains to hold. 
On the other hand, $|Y^{(n)}_{t_i}| / n \rightarrow 0$ for all $1 \leq i \leq |\vermark|$ and $\bu_n(t_i) / n \rightarrow \pi_{t_i}$; hence, subtracting $\norm{\bm_n}_1 \log n$ from both sides, dividing by $n$,  taking limsup over $n$ and then sending $\epsilon$ to zero, the second term in RHS vanishes and we get  $\bchover'^{(2)}_{\bd, \pi}(\mu) \geq \bchover'^{(1)}_{\bd, \pi}(\mu)$. Changing the order of $\bu_n$ and $\tilde{\bu}_n$, we get $\bchover'^{(2)}_{\bd, \pi}(\mu) =\bchover'^{(1)}_{\bd, \pi}(\mu)$. Substituting $\limsup$ with $\liminf$ we get  $\bchunder'^{(2)}_{\bd, \pi}(\mu) =\bchunder'^{(1)}_{\bd, \pi}(\mu)$. This completes the proof. 
\end{proof}

\subsection{Conditions under which the entropy is $-\infty$}
\label{sec:cond-BC-infty}

In this section, we prove that under any of the three conditions in Theorem~\ref{thm:Gen-BC-entorpy-properties}, the BC entropy is $-\infty$. 
This is  proved in Propositions~\ref{prop:not-unimodular-BC--infty}, \ref{prop:deg-not-match-bch-inf} and \ref{prop:not-tree-ent-inf} below. 

In what follows, for integers $n$ and $m$, let $\mG_{n, m}$ be the set of simple unmarked graphs on the vertex set $\{1, \dots, n\}$ with precisely $m$ edges. Moreover, for $\mu \in \mP(\mG_*)$ and $\epsilon > 0$, let $\mG_{n, m}(\mu, \epsilon)$ be the set of graphs $G \in \mG_{n, m}$ such that $\dlp(U(G), \mu) < \epsilon$.
When $\edgemark$ and $\vermark$ are singletons, $\mGb_*$ reduces to $\mG_*$ and the entropy reduces to the unmarked BC entropy defined in \cite{bordenave2014large}. We denote this unmarked entropy with a ``um'' superscript, i.e. $\bchover^\text{um}$, $\bchunder^\text{um}$ and $\bch^\text{um}$.

For the rest of this section, let $\mu$ be a member of $\mP(\mGb_*)$ such that $0 < \deg_x(\mu) < \infty$ for all $x \in \edgemark$ and $\vtype_t(\mu) > 0$ for all $t \in \vermark$. 

\begin{prop}
  \label{prop:not-unimodular-BC--infty}
  If $\mu$ is not unimodular, we have $\bchover_{\bd, \pi}(\mu) = \bchunder_{\bd, \pi}(\mu)= -\infty$ for any $\bd$ and $\pi$. 
\end{prop}

\begin{proof}
Assume $\bchover_{\bd, \pi}(\mu) > -\infty$ for some $\bd=(d_x)_{x \in \edgemark}$ and $\pi=(\pi_t)_{t \in \vermark}$. The definition of $\bchover_{\bd, \pi}(\mu)$ and a diagonalization argument implies that there exists an $M > -\infty$ together with sequences $\{n_k\}_{k=1}^\infty$, $\{\epsilon_k\}_{k=1}^\infty$, $\{\bm_{n_k}\}_{k=1}^\infty$ and $\{\bu_{n_k}\}_{k=1}^\infty$ such that $\bm_{n_k}(x) / {n_k} \rightarrow d_x$ for all $x \in \edgemark$, $\bu_{n_k}(t)/ n \rightarrow \pi_t$  for all $t \in \vermark$, $n_k \rightarrow \infty$, $\epsilon_k \rightarrow 0$, and for all  $k$ 
\begin{equation*}
  \frac{\log |\mG^{(n_k)}_{\bm_{n_k}, \bu_{n_k}}(\mu, \epsilon_k)| - \norm{\bm_{n_k}}_1 \log n}{n_k} > M.
\end{equation*}
This in particular implies that for all $k$, the set $\mG^{(n_k)}_{\bm_{n_k}, \bu_{n_k}}(\mu, \epsilon_k)$ is not empty. Hence, if $\bG_k$ is an arbitrary member of $\mG^{(n_k)}_{\bm_{n_k}, \bu_{n_k}}(\mu, \epsilon_k)$, since $\epsilon_k \rightarrow 0$, $\dlp(U(\bG_k), \mu) \rightarrow 0$. Since the \LP distance metrizes the topology of weak convergence in $\mGb_*$, this means that $\mu$ is the local weak limit of the sequence of finite graphs $\bG_k$, which is a contradiction with the assumption that $\mu$ is not unimodular. Noting that $\bchunder_{\bd, \pi}(\mu) \leq \bchover_{\bd, \pi}(\mu)$, the proof is complete. 
\end{proof}

\begin{prop}
  \label{prop:deg-not-match-bch-inf}
  For a degree vector $\bd = (d_x)_{x \in \Xi}$ and probability distribution $(\pi_t)_{ t \in \vermark}$ such that $0 < d_x < \infty$ for all $x \in \edgemark$ and $\pi_t > 0$ for all $t \in \vermark$, if  $d_{x^*} \neq \deg_{x^*}(\mu)$ for some $x^* \in \Xi$, or $\pi_{\hat{t}} \neq \vtype_{\hat{t}}(\mu)$ for some $\hat{t} \in \vermark$, we have $\bchover_{\bd, \pi}(\mu) = \bchunder_{\bd, \pi}(\mu) = -\infty$. 
\end{prop}

Before we prove this, we need some notation the following lemmas. The proof of the lemmas are postponed until the end of this section. 

 For a marked graph $\bG$ and a mark $x \in \edgemark$, let $\bG_x$ be the simple unmarked graph with the same vertex set and 
including only the edges in $\bG$ with mark $x$. In other words, we throw away edges with marks different from $x$ and remove edge and vertex marks.
More generally, for a subset $X \subseteq \edgemark$, let $\bG_X$ be the unmarked graph obtained from $\bG$ by removing all edges with mark outside $X$, followed by  removing edge and vertex marks. 
In particular, $\bG_{\edgemark}$ is the unmarked graph  obtained form $\bG$ by removing all vertex and edge marks.
See Figure~\ref{fig:Gx} for an example. 
For $X \subseteq \edgemark$, let $T_X: \mGb_* \rightarrow \mG_*$ that maps $[\bG, o]$ to $[\bG_X, o]$. 
Lemma~\ref{lem:Tx-continuous} below implies that $T_X$ is continuous. 
Moreover, for $\mu \in \mP(\mGb_*)$, let $\mu_X \in \mP(\mG_*)$ be the pushforward of $\mu$ under $T_X$. When $X = \{x\}$ is singleton, we denote $T_X$ and $\mu_X$ by $T_x$ and $\mu_x$, respectively.

\begin{figure}
  \centering
\hfill
  %\begin{minipage}{0.33\linewidth}
\subfloat[]{
\centering
  \begin{tikzpicture}[scale=0.5]
    \draw[Cyan,thick] (-1,-1.5) -- (0,-0.5) -- (1,-1.5);
    \draw[Cyan,thick] (-1,1.5) -- (0,0.5) -- (1,1.5);
    \draw[Cyan,thick] (0,-0.5) -- (0,0.5);
    \draw[Orange,densely dotted,very thick] (-1,1.5) -- (0,2.5) -- (1,1.5);
    \draw[Orange,densely dotted,very thick] (-1,-1.5) -- (0,-2.5) -- (1,-1.5);

    % \node[Node2] at (0,0.5) {};
    % \node[Node] at (-1,1.5) {};
    % \node[Node] at (1,1.5) {};
    % \node[Node] at (0,2.5) {};
    % \node[Node2] at (0,-0.5) {};
    % \node[Node] at (-1,-1.5) {};
    % \node[Node] at (1,-1.5) {};
    % \node[Node] at (0,-2.5) {};
    \node[Node2,label={left:4}] at (0,0.5) {};
    \node[Node,label={left:2}] at (-1,1.5) {};
    \node[Node,label={right:3}] at (1,1.5) {};
    \node[Node,label={above:1}] at (0,2.5) {};
    \node[Node2,label={left:5}] at (0,-0.5) {};
    \node[Node,label={left:6}] at (-1,-1.5) {};
    \node[Node,label={right:7}] at (1,-1.5) {};
    \node[Node,label={below:8}] at (0,-2.5) {};

  \end{tikzpicture}
%\end{minipage}%
}
\hfill\hfill
\subfloat[]{
\centering
  \begin{tikzpicture}[scale=0.5]
    \draw[thick] (-1,-1.5) -- (0,-0.5) -- (1,-1.5);
    \draw[thick] (-1,1.5) -- (0,0.5) -- (1,1.5);
    \draw[thick] (0,-0.5) -- (0,0.5);
    %\draw[ange,densely dotted,very thick] (-1,1.5) -- (0,2.5) -- (1,1.5);
    %\draw[Orange,densely dotted,very thick] (-1,-1.5) -- (0,-2.5) -- (1,-1.5);

    % \node[Node2] at (0,0.5) {};
    % \node[Node] at (-1,1.5) {};
    % \node[Node] at (1,1.5) {};
    % \node[Node] at (0,2.5) {};
    % \node[Node2] at (0,-0.5) {};
    % \node[Node] at (-1,-1.5) {};
    % \node[Node] at (1,-1.5) {};
    % \node[Node] at (0,-2.5) {};
    \node[Node,label={left:4},inner sep=1pt] at (0,0.5) {};
    \node[Node,label={left:2},inner sep=1pt] at (-1,1.5) {};
    \node[Node,label={right:3},inner sep=1pt] at (1,1.5) {};
    \node[Node,label={above:1},inner sep=1pt] at (0,2.5) {};
    \node[Node,label={left:5},inner sep=1pt] at (0,-0.5) {};
    \node[Node,label={left:6},inner sep=1pt] at (-1,-1.5) {};
    \node[Node,label={right:7},inner sep=1pt] at (1,-1.5) {};
    \node[Node,label={below:8},inner sep=1pt] at (0,-2.5) {};
  \end{tikzpicture}
%\end{minipage}%
}
\hfill\hfill
\subfloat[]{
\centering
  \begin{tikzpicture}[scale=0.5]
    \draw[thick] (-1,-1.5) -- (0,-0.5) -- (1,-1.5);
    \draw[thick] (-1,1.5) -- (0,0.5) -- (1,1.5);
    \draw[thick] (0,-0.5) -- (0,0.5);
    \draw[thick] (-1,1.5) -- (0,2.5) -- (1,1.5);
    \draw[thick] (-1,-1.5) -- (0,-2.5) -- (1,-1.5);

    % \node[Node2] at (0,0.5) {};
    % \node[Node] at (-1,1.5) {};
    % \node[Node] at (1,1.5) {};
    % \node[Node] at (0,2.5) {};
    % \node[Node2] at (0,-0.5) {};
    % \node[Node] at (-1,-1.5) {};
    % \node[Node] at (1,-1.5) {};
    % \node[Node] at (0,-2.5) {};
    \node[Node,label={left:4},inner sep=1pt] at (0,0.5) {};
    \node[Node,label={left:2},inner sep=1pt] at (-1,1.5) {};
    \node[Node,label={right:3},inner sep=1pt] at (1,1.5) {};
    \node[Node,label={above:1},inner sep=1pt] at (0,2.5) {};
    \node[Node,label={left:5},inner sep=1pt] at (0,-0.5) {};
    \node[Node,label={left:6},inner sep=1pt] at (-1,-1.5) {};
    \node[Node,label={right:7},inner sep=1pt] at (1,-1.5) {};
    \node[Node,label={below:8},inner sep=1pt] at (0,-2.5) {};
  \end{tikzpicture}
%\end{minipage}%
}
\hfill
\caption{\label{fig:Gx} 
(a) A marked graph $\bG$ with  $\edgemark = \{\text{\color{Cyan} Cyan (solid)}, \text{\color{Orange} Orange (dotted)} \}$ and 
$\vermark = \{\bullet, \blacksquare\}$.
(b) $\bG_{\text{\color{Cyan} Cyan}}$, which is obtained from $\bG$ by includes edges with mark {\color{Cyan} Cyan} and removing vertex and edges marks. 
(c) $\bG_{\edgemark}$ which is obtained from $\bG$ by removing all vertex and edge marks.
}
\end{figure}

\begin{lem}
  \label{lem:Tx-continuous}
Let $X \subseteq \edgemark$. Then, for two rooted marked graphs $[\bG, o]$ and $[\bG', o']$ in $\mGb_*$, $d_*([\bG_X, o], [\bG'_X, o']) \leq \bar{d}_*([\bG, o], [\bG', o'])$.
\end{lem}

\begin{lem}
  \label{lem:Gnmn-Tx}
Fix $\mu \in \mP(\mGb_*)$, integer $n$ and vectors $(\bm_n(x))_{x \in \edgemark}$ and $(\bu_n(t))_{t \in \vermark}$. Then, for any $\epsilon>0$, $\bG \in \mG^{(n)}_{\bm_n, \bu_n}(\mu, \epsilon)$ implies $\bG_X \in \mG_{n, \bm_n(X)}(\mu_X, \epsilon)$ where $\bm_n(X) = \sum_{x \in X} \bm_n(x)$.
\end{lem}

\begin{proof}[Proof of Proposition~\ref{prop:deg-not-match-bch-inf}]
We have already shown in the first paragraph of the proof of Proposition~\ref{prop:bch-invariant-un} that if $\pi_{\hat{t}} \neq \vtype_{\hat{t}}(\mu)$ for some $\hat{t} \in \vtype$,  $\bchover_{\bd, \pi}(\mu) = \bchunder_{\bd, \pi}(\mu) = -\infty$. 

Now, assume that $d_{x^*} \neq \deg_{x^*}(\mu)$ for some $x^* \in \edgemark$. 
  Lemma~\ref{lem:Tx-continuous}  shows that $T_x$ is a continuous mapping for all $x \in \edgemark$. 
Fix sequences $(\bm_n(x), x \in \edgemark)$ and $(\bu_n(t), t \in \vermark)$ such that $\bm_n(x) / n \rightarrow d_x / 2$ and $\bu_n(t) / n \rightarrow \pi_t$ for all $x \in \edgemark$ and $t \in \vermark$. 
 Now define the mapping $F_n$ acting on $\mG^{(n)}_{\bm_n, \bu_n}$ that maps $\bG$ to the vector $(\bG_x, x \in \edgemark)$. 
Lemma~\ref{lem:Gnmn-Tx} implies that if $\bG \in \mG^{(n)}_{ \bm_n,\bu_n}(\mu, \epsilon)$,  $\bG_x \in \mG_{n,\bm_n(x)}(\mu_x, \epsilon)$ for all $x \in \edgemark$. 
Note that by having the vector $(\bG_x, x \in \edgemark)$, we can reconstruct edges with correct marks in $\bG$, while the information regarding vertex marks is lost. But there is at most $|\vermark|^n$ possible ways of assigning vertex marks. Hence, 
\begin{equation*}
  \log | \mG^{(n)}_{\bm_n,\bu_n}(\mu, \epsilon)| \leq n \log |\vermark| + \sum_{x \in \edgemark} \log |\mG_{n, \bm_n(x)}(\mu_x, \epsilon)|.
\end{equation*}
Consequently, 
\begin{equation*}
  \begin{split}
    \frac{\log |\mG^{(n)}_{\bm_n,\bu_n}(\mu, \epsilon)| - \norm{\bm_n}_1 \log n}{n} & \leq \log |\vermark| + \frac{\sum_{x \in \edgemark} \log |\mG_{n,\bm_n(x)}(\mu_x, \epsilon) - \bm_n(x) \log n}{n} \\
    &\leq  \log |\vermark| + \frac{\log|\mG_{n, \bm_n(x^*)}(\mu_{x^*}, \epsilon)| - \bm_n(x^*) \log n}{n} \\
    & \qquad + \sum_{x \neq x^*} \frac{\log |\mG_{n, \bm_n(x)}| - \bm_n(x) \log n}{n} \\
    &\leq \frac{\log|\mG_{n, \bm_n(x^*)}(\mu_{x^*}, \epsilon)| - \bm_n(x^*) \log n}{n} + \frac{1}{2} |\edgemark| + \log |\vermark|
  \end{split}
\end{equation*}
where the last inequality uses Lemma~\ref{lem:upper-bound-on-G_n-m_mlogn-n} in Section~\ref{sec:generel-scheme}. Taking limsup from both sides as $n$ goes to infinity, the first term in RHS converges to the unmarked BC entropy of $\mu_{x^*}$ defined in \cite{bordenave2014large}, which we denote by $\bchover_{d_{x^*}}^{\text{um}}(\mu_{d_{x^*}},\epsilon)$. Therefore
\begin{equation*}
  \bchover_{\bd, \pi}(\mu, \epsilon) \leq \bchover_{d_{x^*}}^\text{um}(\mu_{x^*},\epsilon) + \frac{1}{2} |\edgemark| + \log |\vermark|.
\end{equation*}
Now, by sending $\epsilon$ to zero we have 
\begin{equation*}
  \bchover_{\bd, \pi}(\mu) \leq \bchover_{d_{x^*}}^\text{um}(\mu_{x^*}) + \frac{1}{2} |\edgemark| + \log |\vermark|.
\end{equation*}
But, by assumption, $d_{x^*} \neq \deg(\mu_{x^*})$, which together with Theorem~1.2 in \cite{bordenave2014large} implies that the RHS is $-\infty$. 
As a result, $\bchover_{\bd, \pi}(\mu) = -\infty$. 
This together with $\bchunder_{\bd, \pi}(\mu) \leq \bchover_{\bd, \pi}(\mu)$ completes the proof.
\end{proof}

\begin{prop}
  \label{prop:not-tree-ent-inf}
  If the support of $\mu$ is not contained in $\mTb_*$, $\bchunder(\mu)=\bchover(\mu) = -\infty$.
\end{prop}

\begin{proof}
Let $T = T_\edgemark$ be the function that maps $[\bG, o]$ to $[\bG_\edgemark, o]$, which is continuous by  Lemma~\ref{lem:Tx-continuous}. Additionally, let $\bd=(d_x, x \in \edgemark)$ where $d_x = \deg_x(\mu)$ for $x \in \edgemark$, and $\pi=(\pi_t)_{t \in \vermark}$ where $ \pi_t= \vtype_t(\mu)$ for $t \in \vermark$. Moreover, fix sequences $(\bm_n(x))_{ x \in \edgemark}$ and $(\bu_n(t))_{t \in \vermark}$ such that $\bm_n(x) / n \rightarrow d_x /2$ and $\bu_n(t) / n \rightarrow \pi_t$ for all $x \in \edgemark$ and $t \in \vermark$. Furthermore, let $\tilde{\mu} \in \mP(\mG_*)$ be the pushforward of $\mu$ under the mapping $T$. Lemma \ref{lem:Gnmn-Tx} above with $X = \edgemark$ implies that if $\bG \in \mG^{(n)}_{\bm_n, \bu_n}(\mu, \epsilon)$, then $\bG_\edgemark \in \mG_{n, \norm{\bm_n}_1}(\tilde{\mu}, \epsilon)$. However, every graph $\bG_{\edgemark}$ could result from several $\bG$'s, since we are losing information about edge and vertex marks. But there are at most $|\vermark|^n |\edgemark|^{\norm{\bm_n}_1}$ many ways of assigning marks to edges and vertices of $\bG_\edgemark$. Thereby, 
\begin{equation*}
  \frac{\log |\mG^{(n)}_{\bm_n, \bu_n}(\mu, \epsilon)| - \norm{\bm_n}_1 \log n}{n} \leq \frac{\norm{\bm_n}_1 \log |\edgemark|}{n} + \log |\vermark| + \frac{\log |\mG_{n, \norm{\bm_n}_1}(\tilde{\mu}, \epsilon)| - \norm{\bm_n}_1 \log n}{n} 
\end{equation*}
Sending $n$ to infinity and taking limsup,
\begin{equation*}
  \bchover_{\bd, \pi}(\mu, \epsilon) \leq \left ( \sum_{x \in \edgemark} d_x \right ) \log |\edgemark| + \log |\vermark| + \bchover^\text{um}(\tilde{\mu}, \epsilon),
\end{equation*}
If the support of $\mu$ is not contained in $\mTb_*$, the support of $\tilde{\mu}$ is not contained in $\mT_*$. Then, by Theorem~1.2 in \cite{bordenave2014large}, $\bch^{\text{um}} (\tilde{\mu}) = -\infty$. Therefore, by sending $\epsilon$ to zero in the above inequality and noting that $\bchunder_{\bd, \pi}(\mu) \leq \bchover_{\bd, \pi}(\mu)$, we conclude that $\bchunder(\mu)=\bchover(\mu) = -\infty$. 
\end{proof}

Now we turn to proving Lemmas~\ref{lem:Tx-continuous} and \ref{lem:Gnmn-Tx}.

\begin{proof}[Proof of Lemma~\ref{lem:Tx-continuous}]
  By definition, $\bar{d}_*([\bG, o], [\bG', o']) < \epsilon$ means that for some $k$ with $\frac{1}{1+k} < \epsilon$, $[\bG, o]_k \equiv [\bG', o']_k$. This implies $[\bG_X, o]_k \equiv [\bG'_X, o']_k$, which in particular means that $\bar{d}_*([\bG_X, o], [\bG'_X, o']) < \epsilon$. 
\end{proof}

\begin{proof}[Proof of Lemma~\ref{lem:Gnmn-Tx}]
  Note that indeed $\bG_X$ has $\bm_n(X)$ many edges, so we need to show that $\dlp(U(\bG_X), \mu_X) < \epsilon$. In order to do so, we should prove that for any Borel set $B \subset \mG_*$, we have 
  \begin{subequations}
    \begin{align}
      U(\bG_X)(B) &\leq \mu_X(B^\epsilon) + \epsilon \label{eq:UGx-mux-dlp-1}\\
      \mu_X(B) &\leq U(\bG_X)(B^\epsilon) + \epsilon \label{eq:UGx-mux-dlp-2}
    \end{align}
  \end{subequations}
where $B^\epsilon$ is the $\epsilon$--extension of $B$. 
We claim that
\begin{equation}
  \label{eq:UGx-B-UG-Tx-1-B}
  U(\bG_X)(B) = U(\bG)(T_X^{-1}(B)).
\end{equation}
To see this, note that 
\begin{equation*}
  \begin{split}
    U(\bG)(T_X^{-1}(B)) &= \frac{1}{n} \sum_{i=1}^n \one{[\bG, i] \in T_X^{-1}(B)} \\
    &= \frac{1}{n} \sum_{i=1}^n \one{[\bG_X, i] \in B} \\
    &= U(\bG_X)(B).
  \end{split}
\end{equation*}
Moreover, by the definition of $\mu_X$, we have $\mu_X(B^\epsilon) = \mu(T_X^{-1}(B^\epsilon))$. We claim that $(T_X^{-1}(B))^{\epsilon}  \subset T_X^{-1}(B^\epsilon)$. 
To see this, take some $[\bG,o] \in (T_x^{-1}(B))^\epsilon$. This means there exists $[\bG',o'] \in T_X^{-1}(B)$ such that $\bar{d}_*([\bG, o] , [\bG', o']) < \epsilon$. Lemma~\ref{lem:Tx-continuous} above  implies that $d_*([\bG_X, o], (\bG'_X,o')) < \epsilon$. On the other hand, since $[\bG', o'] \in T_X^{-1}(B)$,  $[\bG'_X, o'] \in B$. Thus $[\bG_X, o] \in B^\epsilon$ and $[\bG, o] \in T_X^{-1}(B^\epsilon)$.  Combining this with \eqref{eq:UGx-B-UG-Tx-1-B},
\begin{equation*}
  \begin{split}
    U(\bG_X)(B) &= U(\bG)(T_X^{-1}(B)) \\
    &\stackrel{(a)}{\leq} \mu((T_X^{-1}(B))^\epsilon) + \epsilon \\
    &\leq \mu(T_X^{-1}(B^\epsilon)) + \epsilon \\
    &= \mu_X(B^\epsilon) + \epsilon
  \end{split}
\end{equation*}
where $(a)$ uses the fact that $\bG \in \mG^{(n)}_{\bm_n,\bu_n}(\mu, \epsilon)$. This finishes the proof of \eqref{eq:UGx-mux-dlp-1}. The proof for \eqref{eq:UGx-mux-dlp-2} is similar. This completes the proof.
\end{proof}

%%% Local Variables: 
%%% mode: latex
%%% TeX-master: "UniversalGraphCompression_arXiv"
%%% End: 
